# Supplementary material for: Benchmarking Machine Learning Techniques with Di-Higgs Production at the LHC
Source: arXiv:2009.06754 source file (2020-09-14)
Supplement: Supplementary file 1 [file appendixA.tex]

\appendix
\section{First Appendix}
Please always give a title also for appendices.
